# Supplementary material for: Testing the Wyart-Cates model for non-Brownian shear thickening using bidisperse suspensions
Source: arXiv:1901.02066 ancillary file (2019-11-26)
Supplement: Supplementary file 1 [file arXiv_SoftMatter_SI.pdf]

# Supplementary Information: Testing the Wyart-Cates model for non-Brownian shear thickening using bidisperse suspensions

Ben M. Guy, Christopher Ness, Michiel Hermes, Laura J. Sawiak, Jin Sun and Wilson C. K. Poon

In Section S1, we include further details of experiments. In Section S2, we show a set of flow curves for a monodisperse suspension showing complex shear thickening behaviour. In Section S3, we include full fits of the extended Wyart-Cates model to our bidisperse simulation data.

## S1 Experimental details

**Obtaining steady-state flow curves** To remove loading history, we first ramped down the imposed shear stress,  $\sigma$ , from some stress  $\sigma_0$  to 0.01 Pa, then back up to  $\sigma_0$ ; we chose  $\sigma_0$  *ad hoc* to be below the onset of shear thickening, e.g., for  $x = 20\%$ ,  $\sigma_0 = 4$  Pa. The rheological data we report in Fig. 3(d) are based on a single upward sweep after this pre-shear protocol. We measured the viscosity  $\eta$  as a function as time  $t$  for 10 s per point, which was sufficient to ensure that  $\eta(t)$  had reached a steady state. We show example viscosity traces in Fig. S1 for a small-particle fraction of  $x = 0.2$ ; the  $\sim \mathcal{O}(1$  s) transient after each step change in the imposed  $\sigma$  is an inertial artefact due to acceleration of the rheometer shaft and tool<sup>1</sup>. In Fig. 3(d), we report the average over the last 2 s at each stress.

**Edge fracture** Samples underwent edge fracture at large  $\sigma$ ; however, the exact mode of fracture, and the critical  $\sigma$  or  $\dot{\gamma}$  at which it occurred, varied between different compositions. In some cases, transient “lumps” appeared at the free surface at  $\sigma \gtrsim 1000$  Pa<sup>2</sup>, which are the likely origin of the noisy signal for  $\sigma = 1780$  Pa in Fig. S1(a). As  $\sigma$  is increased, these lumps eventually detached from the sample, resulting in a catastrophic loss of material and a precipitous drop in the apparent  $\eta(t)$  [2370 Pa in Fig. S1(a)]. Other samples, e.g.,  $x = 1$ , Fig. S1(b), fractured by an inertial instability above a critical shear rate<sup>3,4</sup> resulting in progressive loss of sample and a precipitously dropping  $\eta(t)$  [1330 Pa]. The slowly decreasing viscosity for 1000 Pa in Fig. S1 is a precursor to complete fracture.

We find, in general, that the rheology is no longer reproducible once the sample has fractured. We discard stresses for which  $\eta(t)$  drops rapidly in the 10 s window, i.e.,  $\sigma = 2370$  Pa in Fig. S1(a) and 1330 Pa in Fig. S1(b).

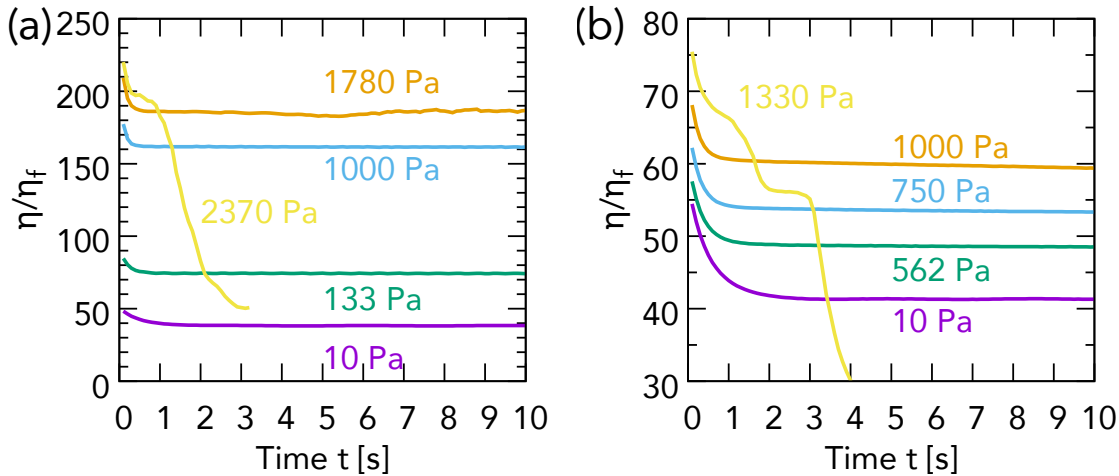

**Fig. S1** Relative viscosity  $\eta/\eta_f$  as a function of time  $t$  for select shear stress  $\sigma$  from the upward  $\sigma$ -sweep used to measure the steady-state flow curves in Fig. 3(d). (a)  $\xi = 0.2$ . (b)  $\xi = 1$ .

**Finite-size effects in bidisperse suspensions** Finally, we observed no evidence of finite-size effects, e.g., intermittent “jamming” of particles in the truncated region of the cone, in either our bidisperse or monodisperse samples (the minimum gap height in our cone-plate setup, in the truncation region, is  $100\mu\text{m} \approx 70d$ ). We observed sporadic jumps in  $\eta$  for measurements in cone-plate and parallel plate geometries with smaller minimum gaps; however, these were not observed for all samples. We will report these data elsewhere.

## S2 Alternative monodisperse shear thickening

Some monodisperse batches of PHSA-stabilised PMMA synthesised in-house exhibited flow curves with two distinct “steps” in the thickening part of the flow curve. Figure S2 shows one such example, for  $d = 3.58\mu\text{m}$  spheres, at different  $\phi$ . Flow curves in the continuous shear thickening regime, e.g., at  $\phi = 0.54$ , exhibit gentle shear thickening above an onset stress  $\sigma_1^* \approx 4\text{Pa}$ , before undergoing an abrupt change in curvature at a higher stress,  $\sigma_2^* \approx 50\text{Pa}$ . This is in contrast to the  $d = 3.78\mu\text{m}$  spheres in Fig. 1(a), which have a comparable diameter but whose  $\eta(\sigma)$  have only a single inflection point. The existence of multiple distinct stress scales in  $\eta(\sigma)$  in Fig. S2 is inconsistent with the single-stress-scale critical-load model used in our simulations.

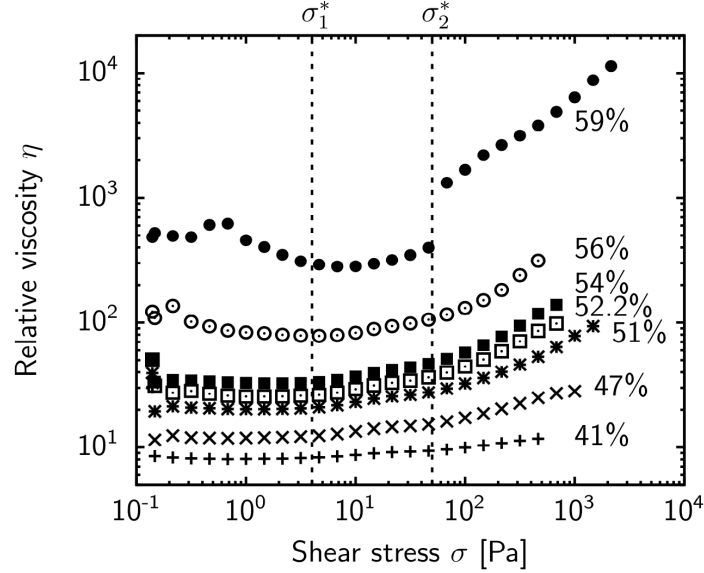

**Fig. S2** *Two-step shear thickening of monodisperse batches* Flow curves  $\eta(\sigma)$  at different  $\phi$  (as labelled) for  $d = 3.58\mu\text{m}$  PHSA-stabilised PMMA in a density-matching CXB-decalin mixture. Data were collected on an Anton Paar MCR301 with a 25 mm-diameter sandblasted cone and sandblasted base plate with an upward shear stress sweep. The waiting time was 30 s per point, to avoid inertial artefacts; we plot averages over the last 5 s. Such behaviour implies an  $f(\sigma)$  that is itself stepped, e.g., due to stepped  $\mu(F)$ .

## S3 Bidisperse Wyart-Cates model fits

In the main text, we fitted the extended WC model, Eq. 1, 2 and 4, to our bidisperse simulation data for  $\xi = 0.2$  (see Fig. 6). Here, we report fits for all values of  $\xi$  studied. Figure S3 shows the equivalent of Fig. 6 for the other values of  $\xi$ ; the  $\xi = 0.2$  fits have been reproduced here, for completeness. Table S1 lists the best-fit coefficients  $\kappa_{11}$ ,  $\kappa_{12}$  and  $\kappa_{22}$ .

| $\xi$ | $\kappa_{11}$ | $\kappa_{12}$ | $\kappa_{22}$ |
|-------|---------------|---------------|---------------|
| 0     | 1             | 0             | 0             |
| 0.2   | 0.7           | 0.3           | 0             |
| 0.5   | 0.4           | 0.6           | 0             |
| 0.65  | 0.05          | 0.95          | 0             |
| 0.8   | 0             | 0.5           | 0.5           |
| 1     | 0             | 0             | 1             |

**Table S1** Best-fit coefficients for extended WC model.

## Notes and references

- 1 J. Richards, J. Royer, B. Liebchen, B. Guy and W. Poon, *Physical Review Letters*, 2019, **123**, 038004.
- 2 M. Hermes, B. M. Guy, W. C. K. Poon, G. Poy, M. E. Cates and M. Wyart, *J. Rheol.*, 2016, **60**, 905–916.
- 3 B. M. Guy, M. Hermes and W. C. K. Poon, *Phys. Rev. Lett.*, 2015, **115**, 088304.
- 4 R. Tanner and M. Keentok, *Journal of Rheology*, 1983, **27**, 47–57.

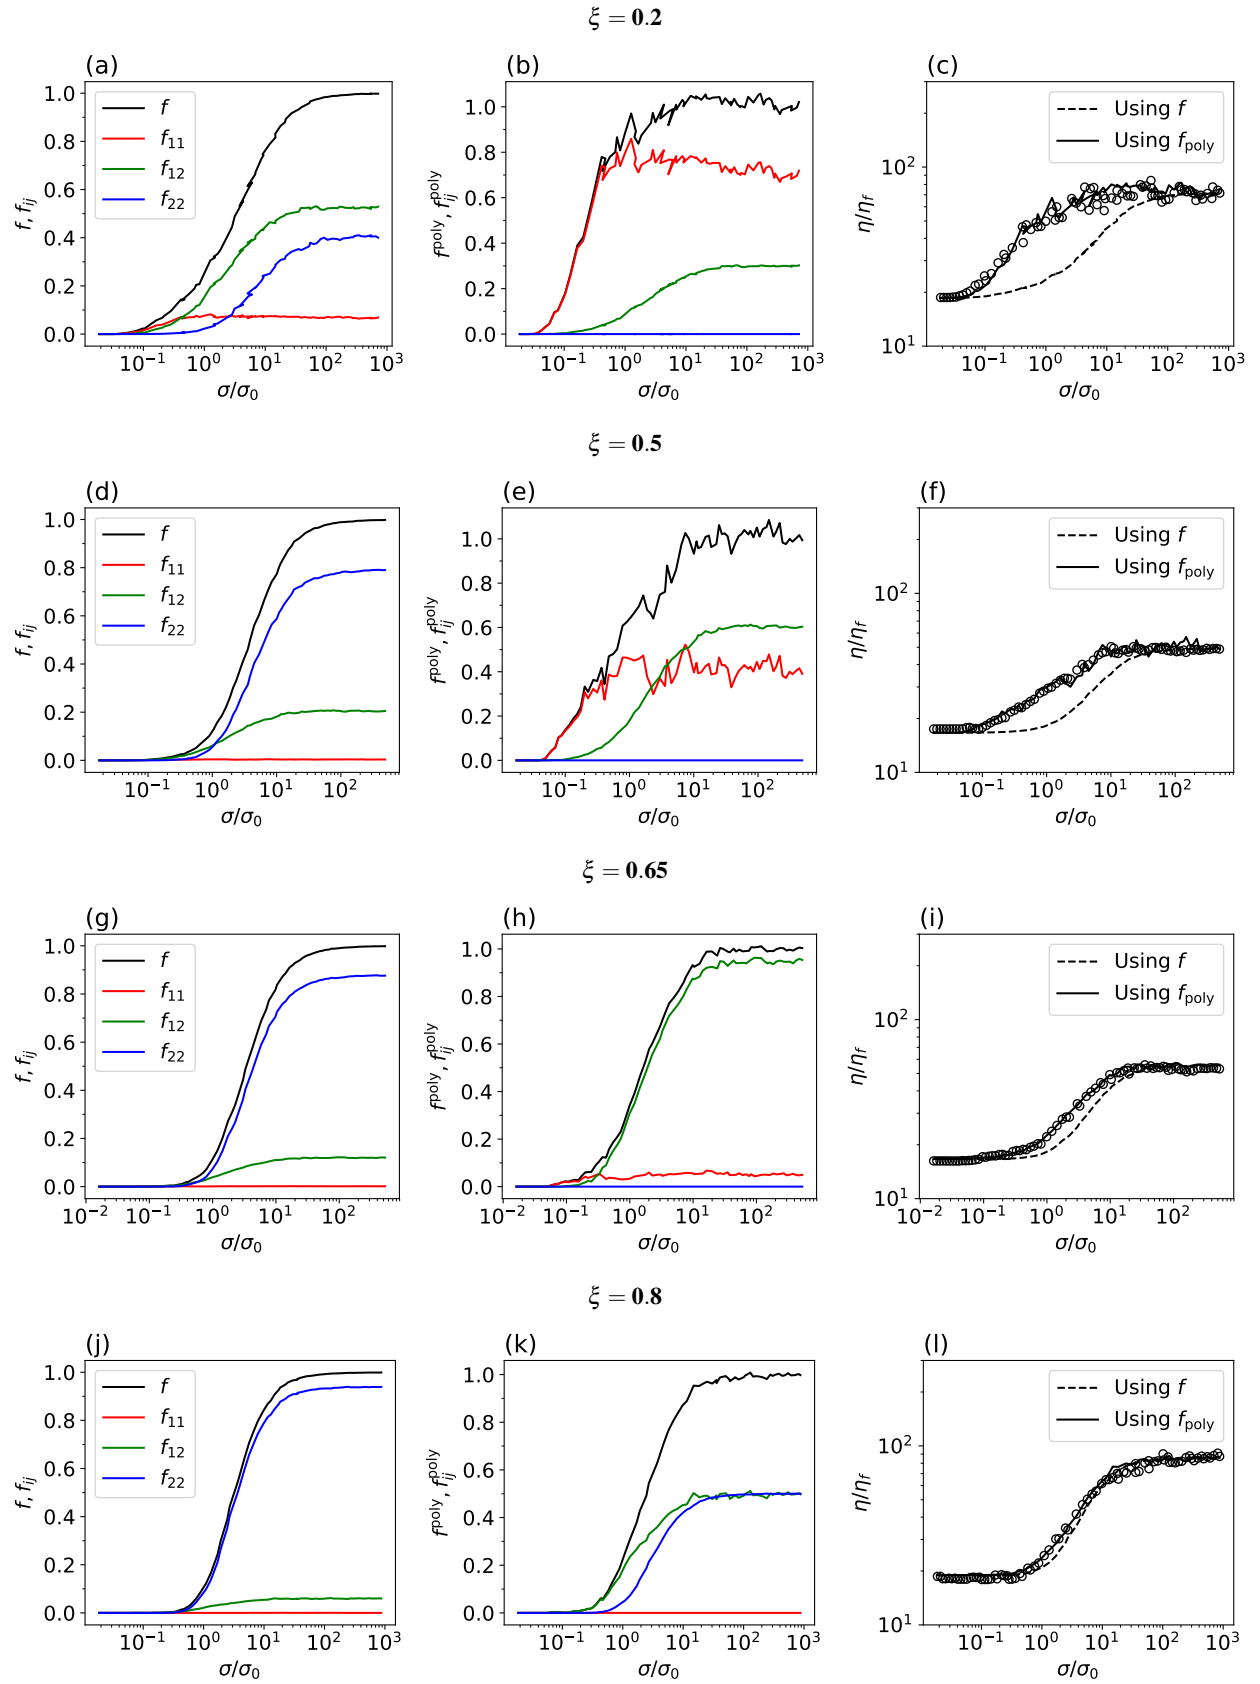

**Fig. S3** Fits of extended WC model to bidisperse simulation flow curves: (a-c)  $\xi = 0.2$ ; (d-f) 0.5; (g-i) 0.65; and (j-l) 0.8. First column, fraction of frictional contacts  $f$  and fractions of large-large (11), large-small (12) and small-small (22) frictional contacts, as labelled. Second column, weighted fractions of frictional contacts; colour scheme the same as in the first column. Third column, simulation flow curves (symbols) with original WC model predictions (dashed line) and fits with the extended WC model (solid lines).
